# Supplementary material for: Distributed Recurrent Neural Forward Models with Synaptic Adaptation for Complex Behaviors of Walking Robots
Source: arXiv:1506.03599 source file (2015-06-11)
Supplement: Supplementary file 1 [file SupplementaryData.pdf]

# Distributed Recurrent Neural Forward Models with Synaptic Adaptation for Complex Behaviors of Walking Robots

## Supplementary Data

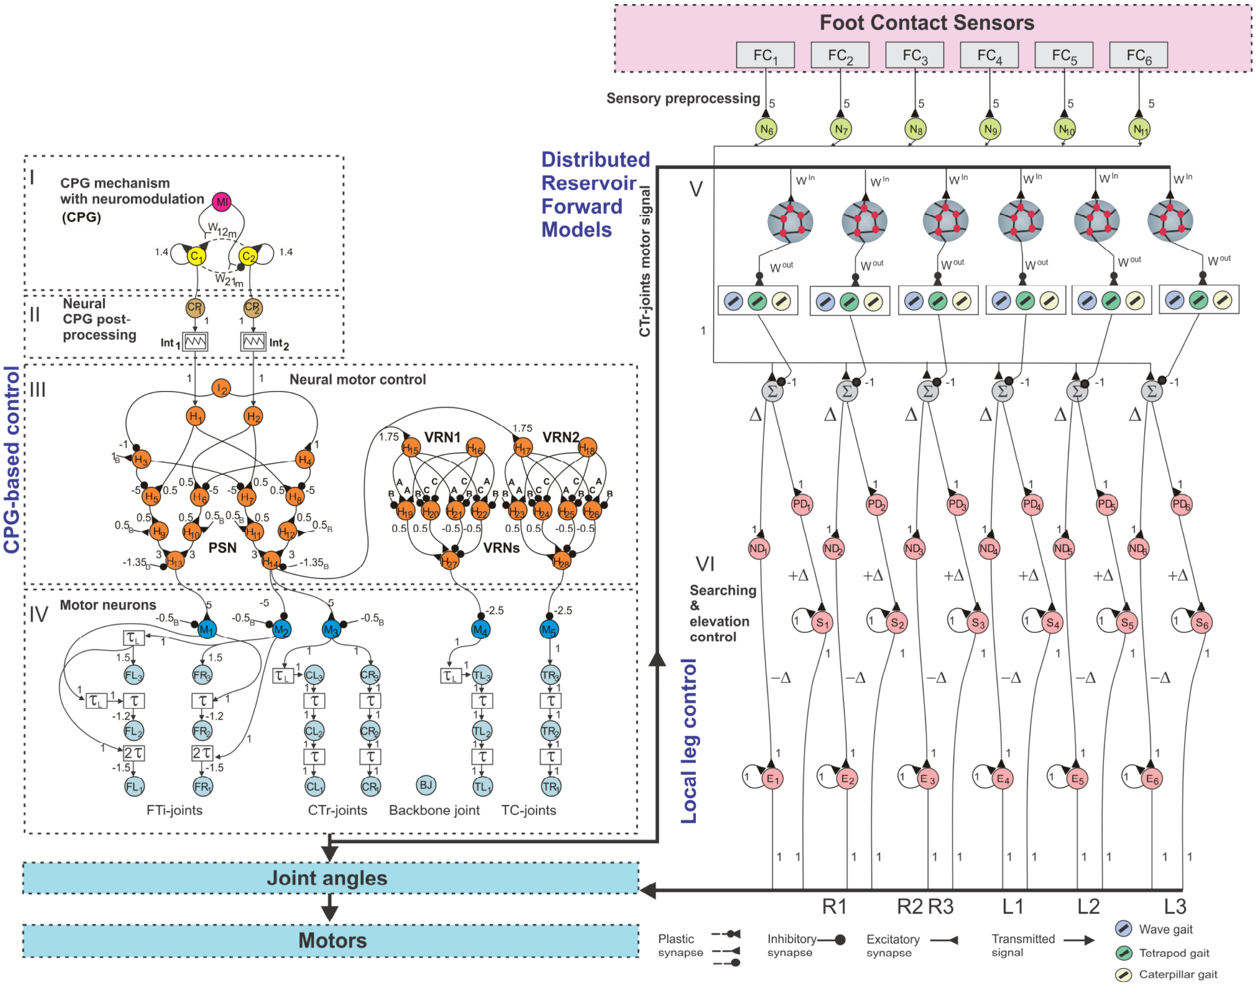


**Figure 1**: **Main wiring diagram of the central pattern generator based control, the reservoir forward models and local leg controls.** Single CPG-based control applied to AMOS II for locomotn. CPG's outputs are projected to PCPG (CPG post processing unit) which translate them into ascending and descending slopes, then these signals are fed to the PSN (phase shift network) component. The outputs of the PSN are projected to the F(R,L) and C(R,L) motor neurons (i.e. the FTi and CTr joints of the robot) through delay lines, as well as to the VRN (velocity regulating network). The VRN's outputs are projected to the T(R,L) motor neurons (TC joints) through delay lines. The CTr joint signals were then used as efference copies that feed as time varying inputs to each of the six reservoir forward models. This in turn is connected to the local searching and elevation controls.

| Parameters | Values |
|---|---|
| Recurrent Network Size – $N$ | $30$ |
| Number of output neurons | $3$ |
| Number of input neurons | $1$ |
| Time step - $\Delta t$ | $0.037$ |
| Neuron time constant initialization - $\tau$ | $10ms$ |
| $\delta_c$ | $10^{-3}$ |
| Scaling parameter - $g$ | $0.95$ |
| Connection probability - $p_c$ | $0.2$ |
| Nonlinearity shape initialization - $a_i$ | $1.0$ |
| Nonlinearity scale initialization - $b_i$ | $0.0$ |
| Auxiliary neuron bias - $B_i$ | $N(0, 0.01)$ |
| Input weight initialization - $W^{in}$ | $U\left[-0.1, 0.1\right]$ |
| Recurrent weight initialization - $W^{rec}$ | $N\left(0, \frac{g^2}{\sqrt{p_c N}}\right)$ |

**Table 1**: **Recurrent Neural Network (reservoir) forward model parameters**
